# Supplementary material for: Impact of irradiation conditions on the magnetic field sensitivity of spin defects in hBN nano flakes
Source: arXiv:2510.13991 source file (2025-10-15)

a)

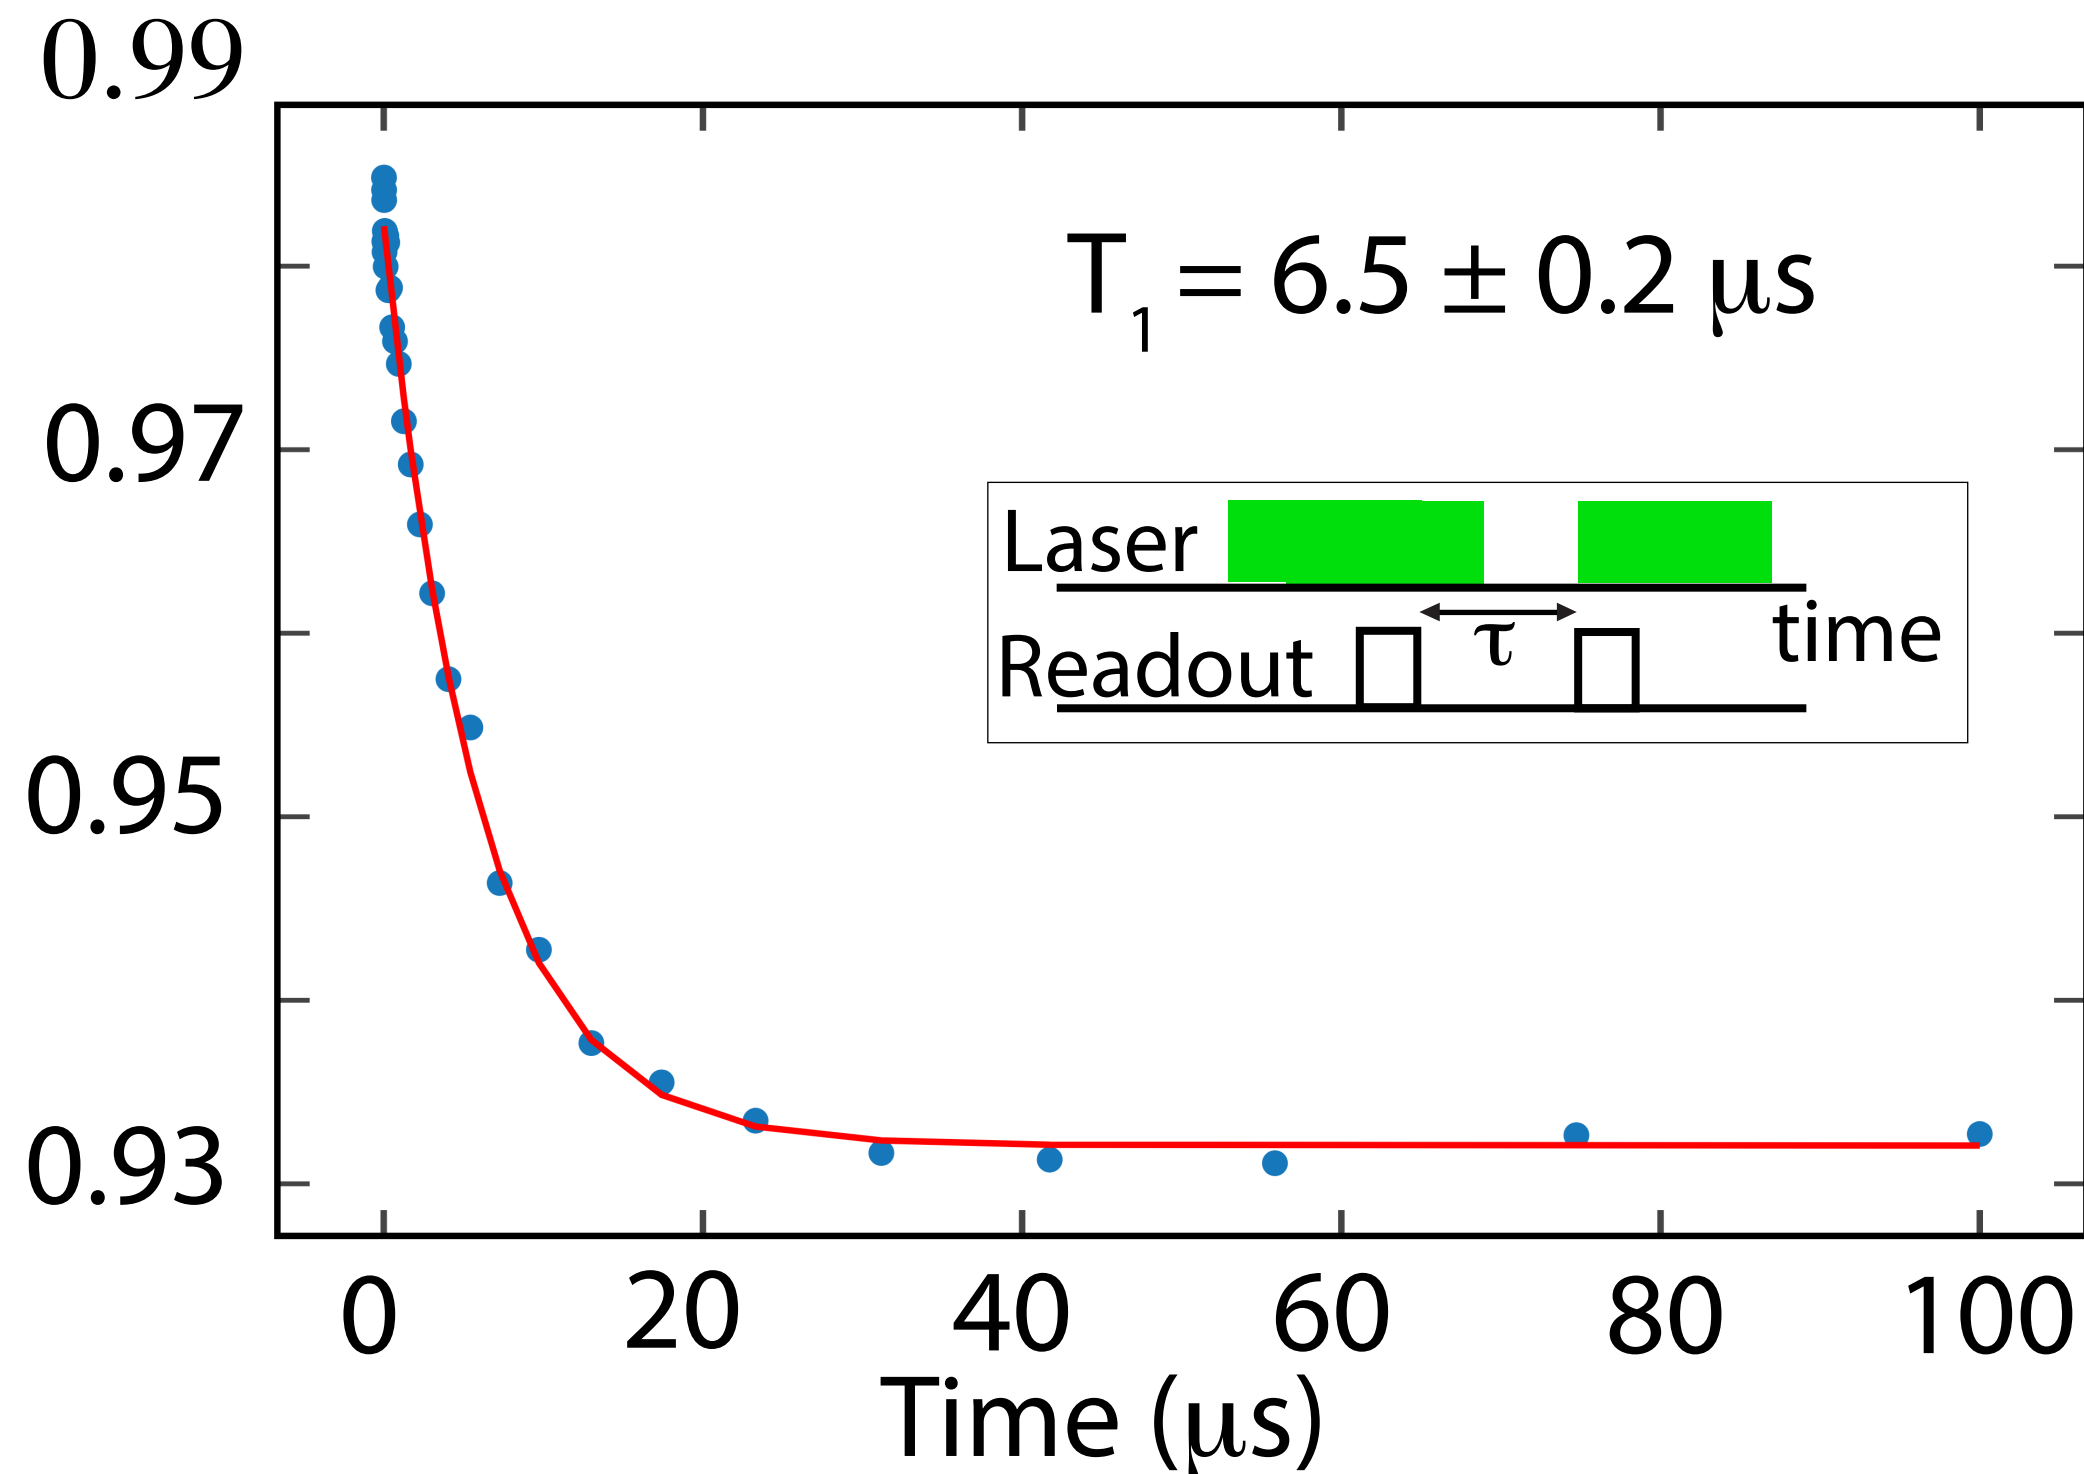

b)

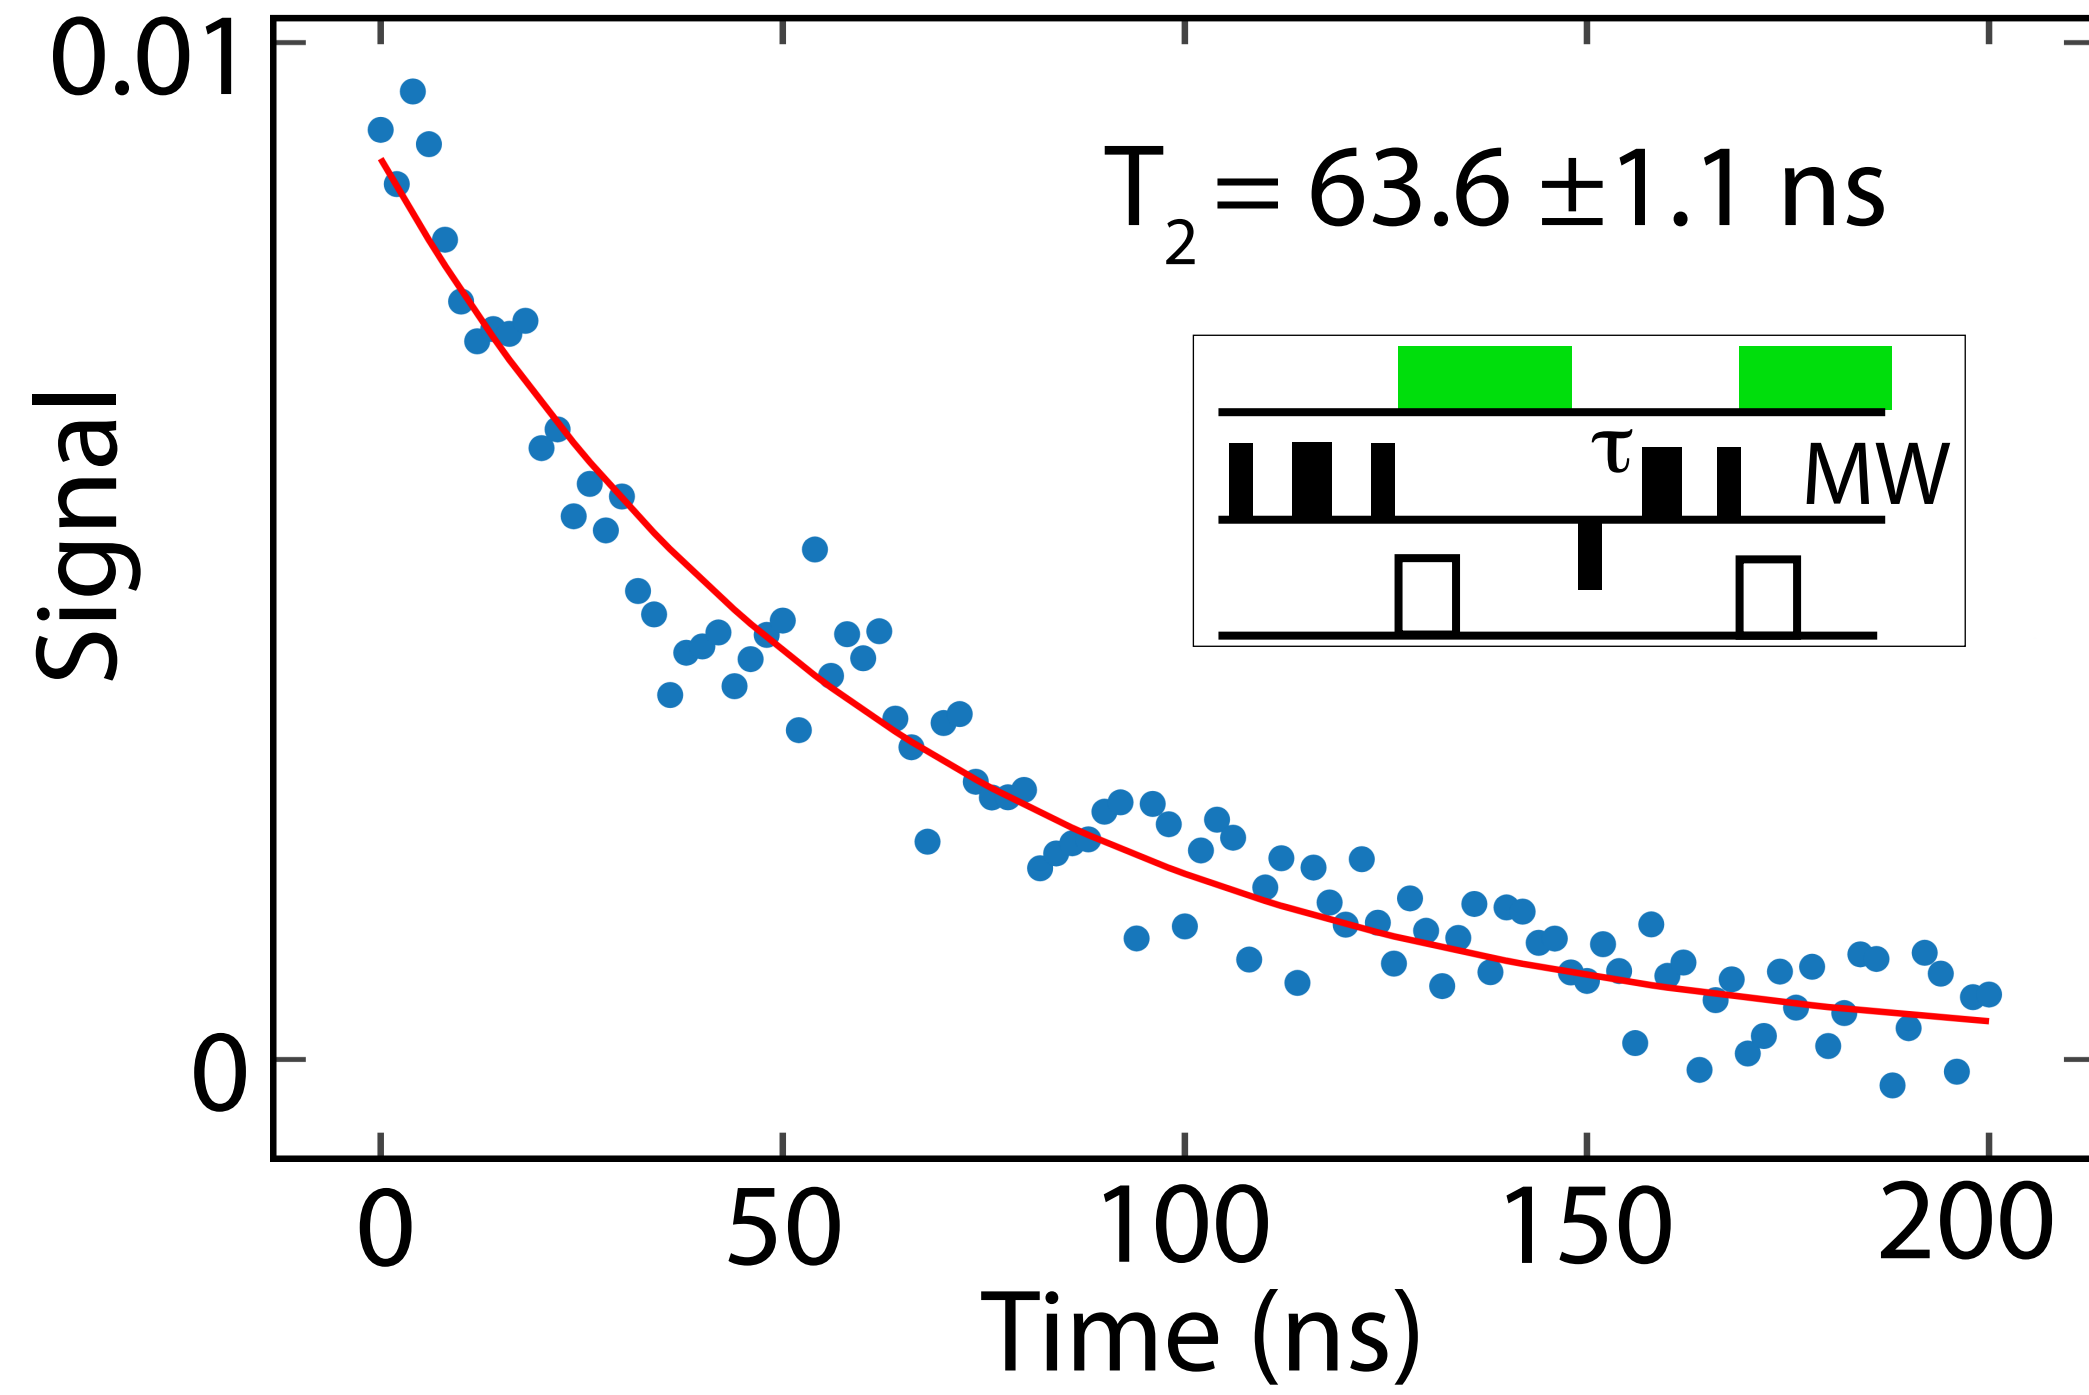

$$T_2 = 63.6 \pm 1.1 \text{ ns}$$

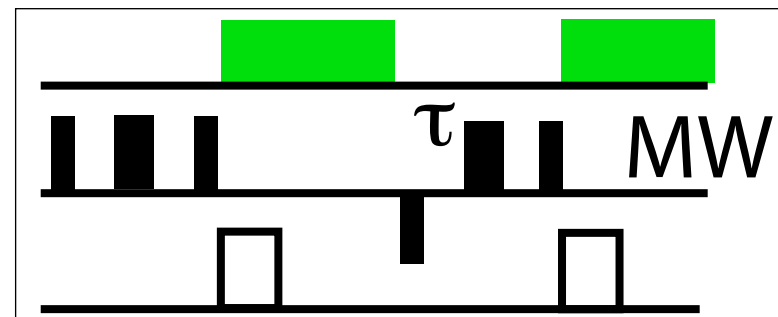

Supplement: Supplementary file 2 [file suppplementaryt1t2.pdf]
